# Supplementary material for: Hydrodynamic theory of chiral angular momentum generation in metals
Source: arXiv:2010.03238 source file (2020-10-07)
Supplement: Supplementary file 1 [file chiral_sm.pdf]

# Supplementary material for
# Hydrodynamic theory of chiral angular momentum generation in metals

Hiroshi Funaki
*5-27-5 Higashiohizumi, Nerima, Tokyo, 178-0063 Japan*

Gen Tatara
*RIKEN Center for Emergent Matter Science (CEMS),
and RIKEN Cluster for Pioneering Research (CPR), 2-1 Hirosawa, Wako, Saitama, 351-0198 Japan*
(Dated: October 7, 2020)

The Hamiltonian we consider is

$$H = \sum_{\boldsymbol{k}} \hat{c}^\dagger_{\boldsymbol{k}} \left(\epsilon_{\boldsymbol{k}} + \boldsymbol{\gamma}_{\boldsymbol{k}} \cdot \boldsymbol{\sigma}\right) \hat{c}_{\boldsymbol{k}} \tag{1}$$

where $\hat{c}$ and $\hat{c}^\dagger$ are electron field operators with two spin components, $\epsilon_{\boldsymbol{k}} \equiv \frac{k^2}{2m} - \epsilon_F$ is the free electron energy ($\epsilon_F$ is the Fermi energy, $m$ is the electron mass). A vector $\boldsymbol{\gamma}_{\boldsymbol{k}}$ represents the spin-orbit interaction, $\boldsymbol{\sigma}$ being a vector of Pauli matrices. We consider the Weyl type,

$$\boldsymbol{\gamma}_{\boldsymbol{k}} = \lambda \boldsymbol{k}, \tag{2}$$

with $\lambda$ a coupling constant. The velocity operator is

$$\hat{v}_i = \frac{k_i}{m} + a_i^\alpha \sigma_\alpha \tag{3}$$

where

$$a_i^\alpha = \frac{d\gamma^\alpha_{\boldsymbol{k}}}{dk_i} = \lambda \delta_{i\alpha} \tag{4}$$

is the anomalous velocity due to the spin-orbit interaction.

## I. MOMENTUM FLUX TENSOR

The explicit expression for the response function for the momentum flux tensor is

$$\pi_{ijk}(\boldsymbol{q}) = \sum_{\boldsymbol{k}} \mathrm{tr}\left[k_i \left(\frac{k_j}{m} + \boldsymbol{a}_j \cdot \boldsymbol{\sigma}\right)\left(f^{\mathrm{r}}_{\boldsymbol{k}-\frac{\boldsymbol{q}}{2}} + h^{\mathrm{r}}_{\boldsymbol{k}-\frac{\boldsymbol{q}}{2}} \hat{\boldsymbol{\gamma}}_{\boldsymbol{k}-\frac{\boldsymbol{q}}{2}} \cdot \boldsymbol{\sigma}\right)\left(\frac{k_k}{m} + \boldsymbol{a}_k \cdot \boldsymbol{\sigma}\right)\left(f^{\mathrm{a}}_{\boldsymbol{k}+\frac{\boldsymbol{q}}{2}} + h^{\mathrm{a}}_{\boldsymbol{k}+\frac{\boldsymbol{q}}{2}} \hat{\boldsymbol{\gamma}}_{\boldsymbol{k}+\frac{\boldsymbol{q}}{2}} \cdot \boldsymbol{\sigma}\right)\right] \tag{5}$$

where ($\lambda = \mathrm{r}, \mathrm{a}$)

$$\begin{aligned} f^\lambda_{\boldsymbol{k}} &\equiv \frac{1}{2}\sum_{\sigma=\pm} g^\lambda_{\boldsymbol{k}\sigma} \\ h^\lambda_{\boldsymbol{k}} &\equiv \frac{1}{2}\sum_{\sigma=\pm} \sigma g^\lambda_{\boldsymbol{k}\sigma} \end{aligned} \tag{6}$$

with

$$g^{\mathrm{r}}_{\boldsymbol{k}\sigma} \equiv \frac{1}{-\epsilon_k - \sigma\gamma_k + \frac{i}{2\tau}} \tag{7}$$

being the diagonalized Green's function, $g^{\mathrm{a}}_{\boldsymbol{k}\sigma} = (g^{\mathrm{r}}_{\boldsymbol{k}\sigma})^*$.

Evaluating the trace in spin, it reduces to

$$\pi_{ijk}(\boldsymbol{q}) = 2\sum_{\boldsymbol{k}}\Bigg[k_i\frac{k_jk_k}{m^2}\left(f^{\rm r}_{\boldsymbol{k}-\frac{\boldsymbol{q}}{2}}f^{\rm a}_{\boldsymbol{k}+\frac{\boldsymbol{q}}{2}}+\left(\hat{\boldsymbol{\gamma}}_{\boldsymbol{k}-\frac{\boldsymbol{q}}{2}}\cdot\hat{\boldsymbol{\gamma}}_{\boldsymbol{k}+\frac{\boldsymbol{q}}{2}}\right)h^{\rm r}_{\boldsymbol{k}+\frac{\boldsymbol{q}}{2}}h^{\rm a}_{\boldsymbol{k}-\frac{\boldsymbol{q}}{2}}\right)$$
$$+\frac{k_i}{m}\left(k_j\boldsymbol{a}_k+k_k\boldsymbol{a}_j\right)\cdot\left(f^{\rm r}_{\boldsymbol{k}-\frac{\boldsymbol{q}}{2}}h^{\rm a}_{\boldsymbol{k}+\frac{\boldsymbol{q}}{2}}\hat{\boldsymbol{\gamma}}_{\boldsymbol{k}+\frac{\boldsymbol{q}}{2}}+f^{\rm a}_{\boldsymbol{k}+\frac{\boldsymbol{q}}{2}}h^{\rm r}_{\boldsymbol{k}-\frac{\boldsymbol{q}}{2}}\hat{\boldsymbol{\gamma}}_{\boldsymbol{k}-\frac{\boldsymbol{q}}{2}}\right)-i\frac{k_i}{m}\left(k_j\boldsymbol{a}_k-k_k\boldsymbol{a}_j\right)\cdot(\hat{\boldsymbol{\gamma}}_{\boldsymbol{k}-\frac{\boldsymbol{q}}{2}}\times\hat{\boldsymbol{\gamma}}_{\boldsymbol{k}+\frac{\boldsymbol{q}}{2}})h^{\rm r}_{\boldsymbol{k}-\frac{\boldsymbol{q}}{2}}h^{\rm a}_{\boldsymbol{k}+\frac{\boldsymbol{q}}{2}}$$
$$+k_i(\boldsymbol{a}_j\cdot\boldsymbol{a}_k)\left(f^{\rm r}_{\boldsymbol{k}-\frac{\boldsymbol{q}}{2}}f^{\rm a}_{\boldsymbol{k}+\frac{\boldsymbol{q}}{2}}-\left(\hat{\boldsymbol{\gamma}}_{\boldsymbol{k}-\frac{\boldsymbol{q}}{2}}\cdot\hat{\boldsymbol{\gamma}}_{\boldsymbol{k}+\frac{\boldsymbol{q}}{2}}\right)h^{\rm r}_{\boldsymbol{k}-\frac{\boldsymbol{q}}{2}}h^{\rm a}_{\boldsymbol{k}+\frac{\boldsymbol{q}}{2}}\right)+ik_i(\boldsymbol{a}_j\times\boldsymbol{a}_k)\cdot(\hat{\boldsymbol{\gamma}}_{\boldsymbol{k}+\frac{\boldsymbol{q}}{2}}f^{\rm r}_{\boldsymbol{k}-\frac{\boldsymbol{q}}{2}}h^{\rm a}_{\boldsymbol{k}+\frac{\boldsymbol{q}}{2}}-\hat{\boldsymbol{\gamma}}_{\boldsymbol{k}-\frac{\boldsymbol{q}}{2}}f^{\rm a}_{\boldsymbol{k}+\frac{\boldsymbol{q}}{2}}h^{\rm r}_{\boldsymbol{k}-\frac{\boldsymbol{q}}{2}})$$
$$+k_i(a^\alpha_ja^\beta_k+a^\alpha_ka^\beta_j)\hat{\gamma}^\alpha_{\boldsymbol{k}-\frac{\boldsymbol{q}}{2}}\hat{\gamma}^\beta_{\boldsymbol{k}+\frac{\boldsymbol{q}}{2}}h^{\rm r}_{\boldsymbol{k}-\frac{\boldsymbol{q}}{2}}h^{\rm a}_{\boldsymbol{k}+\frac{\boldsymbol{q}}{2}}\Bigg] \tag{8}$$

### A. Uniform component ($q = 0$ contribution)

For a linear spin-orbit interaction we consider, $a^\alpha_j$ and $f_{\boldsymbol{k}}$ are even in $\boldsymbol{k}$, while $h_{\boldsymbol{k}}$ is odd. The uniform ($q = 0$) component of the response function is therefore asymmetric with respect to the directions $j$ and $k$ as

$$\pi_{ijk}(0) = -4\sum_{\boldsymbol{k}}k_i(\boldsymbol{a}_j\times\boldsymbol{a}_k)\cdot\hat{\boldsymbol{\gamma}}_{\boldsymbol{k}}{\rm Im}(f^{\rm r}_{\boldsymbol{k}}h^{\rm a}_{\boldsymbol{k}})\equiv\epsilon_{jkl}c_{il} \tag{9}$$

*a. Weyl case* For Weyl type, we have

$$a^\alpha_j = \lambda\delta_{i\alpha}, \qquad \hat{\boldsymbol{\gamma}}_{\boldsymbol{k}} = \hat{\boldsymbol{k}} \tag{10}$$

and $(\boldsymbol{a}_j\times\boldsymbol{a}_k)\cdot\boldsymbol{\gamma}_{\boldsymbol{k}} = \lambda^2\epsilon_{jkl}\hat{\boldsymbol{k}}_l$. We thus have

$$\pi_{ijk}(0) = -\epsilon_{ijk}c \tag{11}$$

where

$$c = -\frac{4}{3}\lambda^2\sum_{\boldsymbol{k}}k{\rm Im}(f^{\rm r}_{\boldsymbol{k}}h^{\rm a}_{\boldsymbol{k}}) = \frac{8}{3}\lambda^2\sum_{\boldsymbol{k}}k{\rm Im}[g^{\rm r}_{k-}g^{\rm a}_{+}] \tag{12}$$

is the bulk chirality coefficient of Weyl system.

*b. Rashba case* For Rashba spin-orbit interaction with the Rashba vector $\boldsymbol{\alpha}$, we have

$$a^\alpha_j = \alpha_\beta\epsilon_{j\alpha\beta}, \qquad \hat{\boldsymbol{\gamma}}_{\boldsymbol{k}} = (\boldsymbol{\alpha}\times\boldsymbol{k})/\gamma_{\boldsymbol{k}} \tag{13}$$

Thus $(\boldsymbol{a}_j\times\boldsymbol{a}_k)\cdot\boldsymbol{\gamma}_{\boldsymbol{k}} = \epsilon_{j\alpha\beta}\epsilon_{k\gamma\delta}\epsilon_{\beta\delta l}\alpha_\alpha\alpha_\gamma(\boldsymbol{\alpha}\times\boldsymbol{k})_l = (\delta_{j\delta}\delta_{\alpha l}-\delta_{jl}\delta_{\alpha\delta})\epsilon_{k\gamma\delta}\alpha_\alpha\alpha_\gamma(\boldsymbol{\alpha}\times\boldsymbol{k})_l = 0$, and uniform component vanishes.

Dresselhaus interaction also leads to a vanishing bulk chiral coefficient.

### B. Viscocity ($q$-linear terms)

$q$-linear terms of $\sigma_{ijk}$, $\sigma^{(1)}_{ijk}$, represents viscosity of the fluid. We expand $\pi_{ijk}(\boldsymbol{q})$ with respect to $\boldsymbol{q}$ to the linear order using

$$f^{\rm r}_{\boldsymbol{k}-\frac{\boldsymbol{q}}{2}}f^{\rm a}_{\boldsymbol{k}+\frac{\boldsymbol{q}}{2}} = f^{\rm r}_{\boldsymbol{k}}f^{\rm a}_{\boldsymbol{k}}+\frac{q_l}{2}(f^{\rm r}_{\boldsymbol{k}}\overleftrightarrow{\partial}_{k_l}f^{\rm a}_{\boldsymbol{k}})+O(q^2) \tag{14}$$

The linear order contribution is then

$$\pi^{(1)}_{ijk}(\boldsymbol{q}) = \sum_{\boldsymbol{k}}q_l\Bigg[\frac{1}{m^2}k_ik_jk_k(f^{\rm r}_{\boldsymbol{k}}\overleftrightarrow{\partial}_{k_l}f^{\rm a}_{\boldsymbol{k}}+\hat{\gamma}^\alpha_{\boldsymbol{k}}h^{\rm r}_{\boldsymbol{k}}\overleftrightarrow{\partial}_{k_l}\hat{\gamma}^\alpha_{\boldsymbol{k}}h^{\rm a}_{\boldsymbol{k}})+\frac{1}{m}k_i\left(k_ja^\alpha_k+k_ka^\alpha_j\right)\left(f^{\rm r}_{\boldsymbol{k}}\overleftrightarrow{\partial}_{k_l}\hat{\gamma}^\alpha_{\boldsymbol{k}}h^{\rm a}_{\boldsymbol{k}}-{\rm c.c.}\right)$$
$$+k_i(\boldsymbol{a}_j\cdot\boldsymbol{a}_k)(f^{\rm r}_{\boldsymbol{k}}\overleftrightarrow{\partial}_{k_l}f^{\rm a}_{\boldsymbol{k}}-\hat{\gamma}^\alpha_{\boldsymbol{k}}h^{\rm r}_{\boldsymbol{k}}\overleftrightarrow{\partial}_{k_l}\hat{\gamma}^\alpha_{\boldsymbol{k}}h^{\rm a}_{\boldsymbol{k}})+k_i(a^\alpha_ja^\beta_k+a^\alpha_ka^\beta_j)(\hat{\gamma}^\alpha_{\boldsymbol{k}}h^{\rm r}_{\boldsymbol{k}}\overleftrightarrow{\partial}_{k_l}\hat{\gamma}^\beta_{\boldsymbol{k}}h^{\rm a}_{\boldsymbol{k}})\Bigg] \tag{15}$$

Derivatives are written using

$$\partial_{k_l}\hat{\gamma}^{\alpha}_{\boldsymbol{k}} = \frac{1}{\gamma_{\boldsymbol{k}}}(\boldsymbol{a}_l - \hat{\boldsymbol{\gamma}}_{\boldsymbol{k}}(\hat{\boldsymbol{\gamma}}_{\boldsymbol{k}}\cdot\boldsymbol{a}_l))_\alpha \tag{16}$$

as

$$\begin{aligned}\partial_{k_l} f^{\rm a}_{\boldsymbol{k}} &= \frac{1}{2}\sum_\sigma\left(\frac{k_l}{m}+\sigma\hat{\boldsymbol{\gamma}}_{\boldsymbol{k}}\cdot\boldsymbol{a}_l\right)(g^{\rm a}_{\boldsymbol{k}\sigma})^2 = \frac{k_l}{m}f^{\rm a(2)}_{\boldsymbol{k}} + (\hat{\boldsymbol{\gamma}}_{\boldsymbol{k}}\cdot\boldsymbol{a}_l)h^{\rm a(2)}_{\boldsymbol{k}} \\ \partial_{k_l}(\hat{\gamma}^{\alpha}_{\boldsymbol{k}}h^{\rm a}_{\boldsymbol{k}}) &= (\partial_{k_l}\hat{\gamma}^{\alpha}_{\boldsymbol{k}})h^{\rm a}_{\boldsymbol{k}} + \hat{\gamma}^{\alpha}_{\boldsymbol{k}}\partial_{k_l}h^{\rm a}_{\boldsymbol{k}} \\ &= \frac{1}{\gamma_{\boldsymbol{k}}}(\boldsymbol{a}_l - \hat{\boldsymbol{\gamma}}_{\boldsymbol{k}}(\hat{\boldsymbol{\gamma}}_{\boldsymbol{k}}\cdot\boldsymbol{a}_l))_\alpha h^{\rm a}_{\boldsymbol{k}} + \hat{\gamma}^{\alpha}_{\boldsymbol{k}}\left(\frac{k_l}{m}h^{\rm a(2)}_{\boldsymbol{k}} + (\hat{\boldsymbol{\gamma}}_{\boldsymbol{k}}\cdot\boldsymbol{a}_l)f^{\rm a(2)}_{\boldsymbol{k}}\right)\end{aligned} \tag{17}$$

where

$$\begin{aligned} f^{\rm a(n)}_{\boldsymbol{k}} &\equiv \frac{1}{2}\sum_\sigma (g^{\rm a}_{\boldsymbol{k}\sigma})^n \\ h^{\rm a(n)}_{\boldsymbol{k}} &\equiv \frac{1}{2}\sum_\sigma \sigma(g^{\rm a}_{\boldsymbol{k}\sigma})^n \end{aligned} \tag{18}$$

We have therefore

$$\begin{aligned} f^{\rm r}_{\boldsymbol{k}}\overset{\leftrightarrow}{\partial}_{k_l} f^{\rm a}_{\boldsymbol{k}} &= 2i{\rm Im}\left[\frac{k_l}{m}f^{\rm r}_{\boldsymbol{k}}f^{\rm a(2)}_{\boldsymbol{k}} + (\hat{\boldsymbol{\gamma}}_{\boldsymbol{k}}\cdot\boldsymbol{a}_l)f^{\rm r}_{\boldsymbol{k}}h^{\rm a(2)}_{\boldsymbol{k}}\right] = 2i\frac{k_l}{m}{\rm Im}\left[f^{\rm r}_{\boldsymbol{k}}f^{\rm a(2)}_{\boldsymbol{k}} + \frac{m\lambda}{k}f^{\rm r}_{\boldsymbol{k}}h^{\rm a(2)}_{\boldsymbol{k}}\right] \\ \hat{\gamma}^{\alpha}_{\boldsymbol{k}}h^{\rm r}_{\boldsymbol{k}}\overset{\leftrightarrow}{\partial}_{k_l}\hat{\gamma}^{\alpha}_{\boldsymbol{k}}h^{\rm a}_{\boldsymbol{k}} &= 2i{\rm Im}\left[\frac{k_l}{m}h^{\rm r}_{\boldsymbol{k}}h^{\rm a(2)}_{\boldsymbol{k}} + (\hat{\boldsymbol{\gamma}}_{\boldsymbol{k}}\cdot\boldsymbol{a}_l)h^{\rm r}_{\boldsymbol{k}}f^{\rm a(2)}_{\boldsymbol{k}}\right] = 2i\frac{k_l}{m}{\rm Im}\left[\overline{h}^{\rm r}_{\boldsymbol{k}}\overline{h}^{\rm a(2)}_{\boldsymbol{k}} + \frac{m\lambda}{k}\overline{h}^{\rm r}_{\boldsymbol{k}}f^{\rm a(2)}_{\boldsymbol{k}}\right] \\ f^{\rm r}_{\boldsymbol{k}}\overset{\leftrightarrow}{\partial}_{k_l}\hat{\gamma}^{\alpha}_{\boldsymbol{k}}h^{\rm a}_{\boldsymbol{k}} &= \frac{1}{\gamma_{\boldsymbol{k}}}[\boldsymbol{a}_l - \hat{\boldsymbol{\gamma}}_{\boldsymbol{k}}(\hat{\boldsymbol{\gamma}}_{\boldsymbol{k}}\cdot\boldsymbol{a}_l)]_\alpha f^{\rm r}_{\boldsymbol{k}}h^{\rm a}_{\boldsymbol{k}} + \hat{\gamma}^{\alpha}_{\boldsymbol{k}}\left[\frac{k_l}{m}(f^{\rm r}_{\boldsymbol{k}}h^{\rm a(2)}_{\boldsymbol{k}} - f^{\rm r(2)}_{\boldsymbol{k}}h^{\rm a}_{\boldsymbol{k}}) + (\hat{\boldsymbol{\gamma}}_{\boldsymbol{k}}\cdot\boldsymbol{a}_l)(f^{\rm r}_{\boldsymbol{k}}f^{\rm a(2)}_{\boldsymbol{k}} - h^{\rm r(2)}_{\boldsymbol{k}}h^{\rm a}_{\boldsymbol{k}})\right] \\ &= \frac{\lambda}{\gamma_{\boldsymbol{k}}}[\delta_{l\alpha} - \hat{k}_\alpha\hat{k}_l]f^{\rm r}_{\boldsymbol{k}}h^{\rm a}_{\boldsymbol{k}} + \frac{\hat{k}_l\hat{k}_\alpha}{m}\left[f^{\rm r}_{\boldsymbol{k}}h^{\rm a(2)}_{\boldsymbol{k}} - f^{\rm r(2)}_{\boldsymbol{k}}h^{\rm a}_{\boldsymbol{k}} + \frac{m\lambda}{k}(f^{\rm r}_{\boldsymbol{k}}f^{\rm a(2)}_{\boldsymbol{k}} - h^{\rm r(2)}_{\boldsymbol{k}}h^{\rm a}_{\boldsymbol{k}})\right]\end{aligned} \tag{19}$$

for the Weyl case. The asymmetric contribution for Weyl case is found to be

$$\pi^{(1){\rm a}}_{ijk} = i\frac{\lambda^2}{3m}(\delta_{ik}q_j - \delta_{jk}q_i){\rm Im}\sum_{\boldsymbol{k}}k^2\left[\frac{1}{\gamma_{\boldsymbol{k}}}f^{\rm r}_{\boldsymbol{k}}h^{\rm a}_{\boldsymbol{k}} + \left(f^{\rm r}_{\boldsymbol{k}}f^{\rm a(2)}_{\boldsymbol{k}} - h^{\rm r}_{\boldsymbol{k}}h^{\rm a(2)}_{\boldsymbol{k}} + \frac{m\lambda}{k}(f^{\rm r}_{\boldsymbol{k}}h^{\rm a(2)}_{\boldsymbol{k}} - h^{\rm r}_{\boldsymbol{k}}f^{\rm a(2)}_{\boldsymbol{k}})\right)\right] \tag{20}$$

In the case of Rashba interaction, antisymmetric components of viscosity is finite due to the anisotropic propagataion, resulting in $\pi^{(1){\rm a}}_{ij} = \pi^{(1){\rm a}}_{ijk}E_k \propto i(q_i\alpha_j - q_j\alpha_i)(\boldsymbol{\alpha}\cdot\boldsymbol{E})$ and $i(\alpha_iE_j - \alpha_jE_i)(\boldsymbol{q}\cdot\boldsymbol{\alpha})$.

Antisymmetric viscosity arises in the presence of anomalous velocity $(\boldsymbol{a}_i\cdot\boldsymbol{\sigma})$, as it requires non-collinear alignment of momentum and velocity.

## II. CONDUCTIVITY

The correlation function $\sigma$ for the conductivity is

$$\begin{aligned}\sigma_{jk}(\boldsymbol{q}) = 2\sum_{\boldsymbol{k}}\Bigg[&\frac{k_jk_k}{m^2}\left(f^{\rm r}_{\boldsymbol{k}-\frac{\boldsymbol{q}}{2}}f^{\rm a}_{\boldsymbol{k}+\frac{\boldsymbol{q}}{2}} + \left(\hat{\boldsymbol{\gamma}}_{\boldsymbol{k}-\frac{\boldsymbol{q}}{2}}\cdot\hat{\boldsymbol{\gamma}}_{\boldsymbol{k}+\frac{\boldsymbol{q}}{2}}\right)h^{\rm r}_{\boldsymbol{k}+\frac{\boldsymbol{q}}{2}}h^{\rm a}_{\boldsymbol{k}-\frac{\boldsymbol{q}}{2}}\right) \\ &+\frac{1}{m}(k_j\boldsymbol{a}_k + k_k\boldsymbol{a}_j)\cdot\left(\hat{\boldsymbol{\gamma}}_{\boldsymbol{k}+\frac{\boldsymbol{q}}{2}}f^{\rm r}_{\boldsymbol{k}-\frac{\boldsymbol{q}}{2}}h^{\rm a}_{\boldsymbol{k}+\frac{\boldsymbol{q}}{2}} + \hat{\boldsymbol{\gamma}}_{\boldsymbol{k}-\frac{\boldsymbol{q}}{2}}f^{\rm a}_{\boldsymbol{k}+\frac{\boldsymbol{q}}{2}}h^{\rm r}_{\boldsymbol{k}-\frac{\boldsymbol{q}}{2}}\right) - i\frac{1}{m}(k_j\boldsymbol{a}_k - k_k\boldsymbol{a}_j)\cdot\left(\hat{\boldsymbol{\gamma}}_{\boldsymbol{k}-\frac{\boldsymbol{q}}{2}}\times\hat{\boldsymbol{\gamma}}_{\boldsymbol{k}+\frac{\boldsymbol{q}}{2}}\right)h^{\rm r}_{\boldsymbol{k}-\frac{\boldsymbol{q}}{2}}h^{\rm a}_{\boldsymbol{k}+\frac{\boldsymbol{q}}{2}} \\ &+(\boldsymbol{a}_j\cdot\boldsymbol{a}_k)\left(f^{\rm r}_{\boldsymbol{k}-\frac{\boldsymbol{q}}{2}}f^{\rm a}_{\boldsymbol{k}+\frac{\boldsymbol{q}}{2}} - \left(\hat{\boldsymbol{\gamma}}_{\boldsymbol{k}-\frac{\boldsymbol{q}}{2}}\cdot\hat{\boldsymbol{\gamma}}_{\boldsymbol{k}+\frac{\boldsymbol{q}}{2}}\right)h^{\rm r}_{\boldsymbol{k}-\frac{\boldsymbol{q}}{2}}h^{\rm a}_{\boldsymbol{k}+\frac{\boldsymbol{q}}{2}}\right) + i(\boldsymbol{a}_j\times\boldsymbol{a}_k)\cdot(\hat{\boldsymbol{\gamma}}_{\boldsymbol{k}+\frac{\boldsymbol{q}}{2}}f^{\rm r}_{\boldsymbol{k}-\frac{\boldsymbol{q}}{2}}h^{\rm a}_{\boldsymbol{k}+\frac{\boldsymbol{q}}{2}} - \hat{\boldsymbol{\gamma}}_{\boldsymbol{k}-\frac{\boldsymbol{q}}{2}}f^{\rm a}_{\boldsymbol{k}+\frac{\boldsymbol{q}}{2}}h^{\rm r}_{\boldsymbol{k}-\frac{\boldsymbol{q}}{2}}) \\ &+(a^\alpha_ja^\beta_k + a^\alpha_ka^\beta_j)\hat{\gamma}^\alpha_{\boldsymbol{k}-\frac{\boldsymbol{q}}{2}}\hat{\gamma}^\beta_{\boldsymbol{k}+\frac{\boldsymbol{q}}{2}}h^{\rm r}_{\boldsymbol{k}-\frac{\boldsymbol{q}}{2}}h^{\rm a}_{\boldsymbol{k}+\frac{\boldsymbol{q}}{2}}\Bigg]\end{aligned} \tag{21}$$

The antisymmetric component is induced by the chiral nature is

$$\sigma^{\rm a}_{jk}(\boldsymbol{q}) = 2i\sum_{\boldsymbol{k}}\left[-\frac{1}{m}\left(k_j\boldsymbol{a}_k - k_k\boldsymbol{a}_j\right)\cdot\left(\hat{\boldsymbol{\gamma}}_{\boldsymbol{k}-\frac{\boldsymbol{q}}{2}}\times\hat{\boldsymbol{\gamma}}_{\boldsymbol{k}+\frac{\boldsymbol{q}}{2}}\right)h^{\rm r}_{\boldsymbol{k}-\frac{\boldsymbol{q}}{2}}h^{\rm a}_{\boldsymbol{k}+\frac{\boldsymbol{q}}{2}} + (\boldsymbol{a}_j\times\boldsymbol{a}_k)\cdot(\hat{\boldsymbol{\gamma}}_{\boldsymbol{k}+\frac{\boldsymbol{q}}{2}}f^{\rm r}_{\boldsymbol{k}-\frac{\boldsymbol{q}}{2}}h^{\rm a}_{\boldsymbol{k}+\frac{\boldsymbol{q}}{2}} - \hat{\boldsymbol{\gamma}}_{\boldsymbol{k}-\frac{\boldsymbol{q}}{2}}f^{\rm a}_{\boldsymbol{k}+\frac{\boldsymbol{q}}{2}}h^{\rm r}_{\boldsymbol{k}-\frac{\boldsymbol{q}}{2}})\right] \tag{22}$$

We see that the leading order is linear in $\boldsymbol{q}$. Using $(\boldsymbol{a}_j\times\boldsymbol{a}_k)\cdot\boldsymbol{\gamma}_{\boldsymbol{k}} = \lambda^2\epsilon_{jkl}\hat{\boldsymbol{k}}_l$ for Weyl case,

$$\sigma^{\rm a}_{jk} = \sigma^{\rm a}_0\epsilon_{jkl}q_l, \tag{23}$$

where $\sigma^{\rm a}_0$ is a finite constant. This component induces a chiral surface current in the plane perpendicular to the applied electric field, called the anomalous edge current in Ref.[1].

For Rashba case, $(\boldsymbol{a}_j\times\boldsymbol{a}_k)\cdot\boldsymbol{\gamma}_{\boldsymbol{k}} = 0$, $(\boldsymbol{a}_j\times\boldsymbol{a}_k)\cdot\boldsymbol{a}_l = 0$, and asymmetric component vanishes.

## III. INDUCED SPIN

The induced spin due to the applied electric field is represented by a correlation function

$$s_{jk}(\boldsymbol{q}) = \frac{-1}{\Omega}\int\frac{d\omega}{2\pi}\sum_{\boldsymbol{k}}{\rm tr}[\sigma_j G_{\boldsymbol{k}\omega}v_k G_{\boldsymbol{k}+\boldsymbol{q},\omega+\Omega}]^< \tag{24}$$

We consider the ubniform component, which is

$$s_{jk}(0) = \sum_{\boldsymbol{k}}{\rm tr}\left[\sigma_j\left(\frac{k_k}{m}(f^{\rm r}_{\boldsymbol{k}}h^{\rm a}_{\boldsymbol{k}}(\hat{\boldsymbol{\gamma}}_{\boldsymbol{k}}\cdot\boldsymbol{\sigma}) + {\rm c.c.}) + a^l_k\left[\sigma_l f^{\rm r}_{\boldsymbol{k}}f^{\rm a}_{\boldsymbol{k}} + h^{\rm r}_{\boldsymbol{k}}h^{\rm a}_{\boldsymbol{k}}(\hat{\boldsymbol{\gamma}}_{\boldsymbol{k}}\cdot\boldsymbol{\sigma})\sigma_l(\hat{\boldsymbol{\gamma}}_{\boldsymbol{k}}\cdot\boldsymbol{\sigma})\right]\right)\right] \tag{25}$$

For the Weyl case,

$$s_{jk}(0) = 2\delta_{jk}\sum_{\boldsymbol{k}}\left[\frac{k}{3m}(f^{\rm r}_{\boldsymbol{k}}h^{\rm a}_{\boldsymbol{k}} + {\rm c.c.}) + \lambda f^{\rm r}_{\boldsymbol{k}}f^{\rm a}_{\boldsymbol{k}} - \frac{\lambda}{3}h^{\rm r}_{\boldsymbol{k}}h^{\rm a}_{\boldsymbol{k}}\right] \tag{26}$$

## IV. EVALUATION OF SUMMATION OVER $\boldsymbol{k}$ IN $c$ AND $\eta^{\rm a}$

Two chiral coefficients of our interest are

$$\begin{aligned} c &= -\frac{4}{3}\lambda^2\frac{e}{V}\sum_{\boldsymbol{k}}k{\rm Im}(f^{\rm r}_{\boldsymbol{k}}h^{\rm a}_{\boldsymbol{k}}) \\ \eta^{\rm a} &= -\frac{\lambda^2}{3m}{\rm Im}\sum_{\boldsymbol{k}}k^2\left[\frac{1}{\gamma_{\boldsymbol{k}}}f^{\rm r}_{\boldsymbol{k}}h^{\rm a}_{\boldsymbol{k}} + \left(f^{\rm r}_{\boldsymbol{k}}f^{\rm a(2)}_{\boldsymbol{k}} - h^{\rm r}_{\boldsymbol{k}}h^{\rm a(2)}_{\boldsymbol{k}} + \frac{m\lambda}{k}(f^{\rm r}_{\boldsymbol{k}}h^{\rm a(2)}_{\boldsymbol{k}} - h^{\rm r}_{\boldsymbol{k}}f^{\rm a(2)}_{\boldsymbol{k}})\right)\right] \end{aligned} \tag{27}$$

In terms of diagonalized Green's function,

$$\begin{aligned} {\rm Im}(f^{\rm r}_{\boldsymbol{k}}h^{\rm a}_{\boldsymbol{k}}) &= -\frac{1}{2}{\rm Im}[g^{\rm r}_{\boldsymbol{k}+}g^{\rm a}_{\boldsymbol{k}-}] \\ {\rm Im}(f^{\rm r}_{\boldsymbol{k}}f^{\rm a(2)}_{\boldsymbol{k}}) &= \frac{1}{4}\sum_\sigma{\rm Im}[g^{\rm r}_{\boldsymbol{k}\sigma}(g^{\rm a}_{\boldsymbol{k}\sigma})^2 + g^{\rm r}_{\boldsymbol{k}\sigma}(g^{\rm a}_{\boldsymbol{k},-\sigma})^2] \\ {\rm Im}(h^{\rm r}_{\boldsymbol{k}}h^{\rm a(2)}_{\boldsymbol{k}}) &= \frac{1}{4}\sum_\sigma{\rm Im}[g^{\rm r}_{\boldsymbol{k}\sigma}(g^{\rm a}_{\boldsymbol{k}\sigma})^2 - g^{\rm r}_{\boldsymbol{k}\sigma}(g^{\rm a}_{\boldsymbol{k},-\sigma})^2] \\ {\rm Im}(f^{\rm r}_{\boldsymbol{k}}f^{\rm a(2)}_{\boldsymbol{k}} - h^{\rm r}_{\boldsymbol{k}}h^{\rm a(2)}_{\boldsymbol{k}}) &= \frac{1}{2}\sum_\sigma{\rm Im}[g^{\rm r}_{\boldsymbol{k}\sigma}(g^{\rm a}_{\boldsymbol{k},-\sigma})^2] \end{aligned} \tag{28}$$

The summation over $\boldsymbol{k}$ is carried out by use of contour integration. using density of states, $\nu(\epsilon) \propto \sqrt{\epsilon + \epsilon_F}$,

$$\sum_{\boldsymbol{k}} g^{\mathrm{r}}_{\boldsymbol{k}+} g^{\mathrm{a}}_{\boldsymbol{k}-} = \int d\epsilon \nu(\epsilon) \frac{1}{\epsilon + \gamma_\epsilon - \frac{i}{2\tau}} \frac{1}{\epsilon - \gamma_\epsilon + \frac{i}{2\tau}}$$
$$= -\frac{\pi}{2} i \sum_\sigma \frac{\nu_\sigma}{\gamma_\sigma - \frac{i}{2\tau}}$$
$$\sum_{\boldsymbol{k}} g^{\mathrm{r}}_{\boldsymbol{k}+} (g^{\mathrm{a}}_{\boldsymbol{k}-})^2 = -\frac{\pi}{4} i \left[ \sum_\sigma \frac{\nu_\sigma}{(\gamma_\sigma - \frac{i}{2\tau})^2} - \frac{\nu_-}{\gamma_- - \frac{i}{2\tau}} \frac{1}{2\epsilon_-} \right] \tag{29}$$

where $\nu_\sigma$, $\epsilon_\sigma$ and $\gamma_\sigma$ denotes density of states, energy $\epsilon$ and $\gamma_{\boldsymbol{k}}$ evaluated at $k_\sigma$, the Fermi wave vector of spin $\sigma$ state ($k_\sigma \equiv \sqrt{2m(\epsilon_F + \sigma\gamma_\sigma)}$ and $\epsilon_\sigma = \epsilon_F + \sigma\gamma_\sigma$). The imaginary parts are

$$\mathrm{Im} \sum_{\boldsymbol{k}} g^{\mathrm{r}}_{\boldsymbol{k}+} g^{\mathrm{a}}_{\boldsymbol{k}-} = -\frac{\pi}{2} \sum_\sigma \frac{\nu_\sigma \gamma_\sigma}{(\gamma_\sigma)^2 + \frac{1}{4\tau^2}}$$
$$\mathrm{Im} \sum_{\boldsymbol{k}} g^{\mathrm{r}}_{\boldsymbol{k}+} (g^{\mathrm{a}}_{\boldsymbol{k}-})^2 = -\frac{\pi}{4} \left[ \sum_\sigma \frac{\nu_\sigma ((\gamma_\sigma)^2 - \frac{1}{4\tau^2})}{[(\gamma_\sigma)^2 + \frac{1}{4\tau^2}]^2} - \frac{\nu_-}{(\gamma_-)^2 + \frac{1}{4\tau^2}} \frac{\gamma_-}{\epsilon_-} \right] \tag{30}$$

The chiral coefficients are thus

$$c = -\frac{\pi}{3} \frac{e\lambda^2}{a^3} \sum_\sigma \frac{\nu_\sigma \gamma_\sigma k_\sigma}{(\gamma_\sigma)^2 + \frac{1}{4\tau^2}}$$
$$\eta^{\mathrm{a}} = -\frac{\pi e \lambda^2}{24 m a^3} \sum_\sigma \nu_\sigma k_\sigma^2 \left[ \frac{1}{\tau^2} \frac{1}{[(\gamma_\sigma)^2 + \frac{1}{4\tau^2}]^2} + 2 \frac{\gamma_\sigma}{\epsilon_\sigma} \frac{1}{(\gamma_\sigma)^2 + \frac{1}{4\tau^2}} \left( 1 + \sigma \frac{m\lambda}{2k_\sigma} \right) \right] \tag{31}$$

Limit value for clean ($\gamma_\sigma \tau \gg 1$) limit is

$$c \simeq -\frac{\pi}{3} \frac{e\lambda^2}{a^3} \sum_\sigma \frac{\nu_\sigma k_\sigma}{\gamma_\sigma}$$
$$\eta^{\mathrm{a}} \simeq -\frac{\pi e \lambda^2}{24 m a^3} \sum_\sigma \nu_\sigma k_\sigma^2 \frac{1}{\gamma_\sigma \epsilon_\sigma} \left( 1 + \sigma \frac{m\lambda}{2k_\sigma} \right) \tag{32}$$

while

$$c \simeq -\frac{4\pi}{3} \frac{e\lambda^2}{a^3} \sum_\sigma \nu_\sigma \gamma_\sigma k_\sigma \tau^2$$
$$\eta^{\mathrm{a}} \simeq -\frac{2\pi e \lambda^2}{3 m a^3} \sum_\sigma \nu_\sigma k_\sigma^2 \tau^2 \left( 1 + \frac{\gamma_\sigma}{2\epsilon_\sigma} \left( 1 + \sigma \frac{m\lambda}{2k_\sigma} \right) \right) \tag{33}$$

for dirty ($\gamma_\sigma \tau \ll 1$) limit.

The spin density response function is

$$\kappa_s = 2 \frac{e}{V} \sum_{\boldsymbol{k}} \mathrm{Re} \left[ \frac{2k}{3m} f^{\mathrm{r}}_{\boldsymbol{k}} h^{\mathrm{a}}_{\boldsymbol{k}} + \lambda f^{\mathrm{r}}_{\boldsymbol{k}} f^{\mathrm{a}}_{\boldsymbol{k}} - \frac{\lambda}{3} h^{\mathrm{r}}_{\boldsymbol{k}} h^{\mathrm{a}}_{\boldsymbol{k}} \right]$$
$$= \frac{2\pi e}{3a^3} \sum_\sigma \frac{\nu_\sigma}{k_\sigma} \tau \left( \sigma \epsilon_\sigma + \gamma_\sigma \frac{\gamma_\sigma^2 + \frac{3}{8\tau^2}}{\gamma_\sigma^2 + \frac{1}{4\tau^2}} \right) \tag{34}$$

## ACKNOWLEDGMENTS

This study was supported by a Grant-in-Aid for Scientific Research (B) (No. 17H02929) from the Japan Society for the Promotion of Science.

[1] R. Toshio, K. Takasan, and N. Kawakami, Phys. Rev. Research **2**, 032021 (2020).
